# Supplementary material for: Technologies on Effectiveness and Efficiency: A Survey of State Spaces Models
Source: arXiv:2503.11224 source file (2025-03-14)
Supplement: Supplementary file 1 [file 13_appendix.tex]

\section{Symbol Table}

\begin{table}[ht]
\centering
\caption{Symbol Table.}
\begin{tabular}{l|c}
\toprule
\textbf{Symbol} & \textbf{Meaning} \\ 
\midrule
$x$ & input of SSM \\
$y$ & output of SSM \\
$h$ & latent state of SSM \\
$L$ & sequence length \\
% $N$ & input/output dimension \\
% $M$ & latent state dimension \\
% $D$ & (maybe) model dimension \\

\bottomrule
\end{tabular}
\label{tab:stat}
\end{table}
